# Supplementary material for: A Cooperation Graph Approach for Multiagent Sparse Reward Reinforcement Learning
Source: arXiv:2208.03002 source file (2022-08-05)
Supplement: Supplementary file 1 [file additional.tex]

\subsection{???}
\subsubsection{what is this?}
Note that cluster-action needs to be translated back to the original agent-action space,
on the one hand,
this model structure provides a possibility for
designing a different set of actions
above the original action space.
which can describe specific but obvious cooperation foundamental behaviors.
E.g. gathering at a given position for a group of ant-like agents.
Suppose the original action for agents is velocity direction,
a simple target controller translating destination coordinate to velocity direction
is binded to the target node.

From another perspective,
it can be view as a change of decision making subject.
The clusters instead of agents take actions in the Cooperation Graph.
In this way, we introduced a prior knowledge assumption, which indicates that 
cooperative multiagent tasks can be accomplished by
dynamic agent clusters, where agents share the same cluster-actions.
In this approach, we significantly reduced the policy space requires exploration.

With the increase of the team scale, the number of nodes grows linearly while the possible state of the graph grows exponentially.
Besides the complexity, the graph is not static.

\subsection{Bottleneck Creating}
% introduce the relationship of agents, clusters and entities
% why this architachture create a bottleneck in agents exploration
The defination of entity is flexible regrading to different tasks, 
which can be any objects in the environments that an agent can interract, 
grid points in the map, agents itself or even an abstract state.

Action domin transition!

\subsection{Swarm System Extension}
The cluster-based design allows our model to explore multiagent systems with hundreds of agents, with several simple modifications.
The feature of the agent-clustering policy (ACP) is that agents adjust their cluster identity one by one at each time step. As the agent number grows larger, so as the adjustment delay.
It is especially important at the beginning of an episode as the swarm starts from a random cluster distribution. 
In most cases, as an episode starts, 
the model has to reconstruct the existing agent-cluster cooperation graph, which involves many steps of action and is time-costing. 
In contrast,  adjustments in cluster-target connection will become the dominant part of the action, rapidly responding to the varying environment.
We propose a straightforward way to solve the time step problem by 1) allowing multiple action steps to be executed within a time step and 2) 
batching agents when processing the initial agent exchange actions.

The usual practice in reinforcement learning is generating an action signal at each time step. 
Fortunately, our model is built with an internal environment capable of cooperation relationship abstraction and generating trajectories described in intrinsic state space.
Thus it is simple to isolate the flow of the extrinsic time step and the intrinsic action step, 
which is shown in Fig.\ref{}
